# Supplementary material for: Deterministic field-free skyrmion nucleation at a nano-engineered injector device
Source: arXiv:1902.10435 ancillary file (2019-02-27)
Supplement: Supplementary file 1 [file Skyrmion_Nucleation_SI.pdf]

# SUPPLEMENTARY INFORMATION: Deterministic field-free skyrmion nucleation at a nano-engineered injector device

Simone Finizio,[1,*] Katharina Zeissler,[2] Sebastian Wintz,[1,3] Sina Mayr,[1,4] Teresa Weßels,[5] Alexandra J. Huxtable,[2] Gavin Burnell,[2] Christopher H. Marrows,[2] and Jörg Raabe[1]

[1]*Swiss Light Source, Paul Scherrer Institut, 5232 Villigen PSI, Switzerland*

[2]*School of Physics and Astronomy, University of Leeds, Leeds LS2 9JT, United Kingdom*

[3]*Institute of Ion Beam Physics and Materials Research, Helmholtz-Zentrum Dresden-Rossendorf, 01328 Dresden, Germany*

[4]*Department of Materials, Laboratory for Mesoscopic Systems, ETH Zürich, 8093 Zürich, Switzerland*

[5]*Ernst Ruska-Centre for Microscopy and Spectroscopy with Electrons and Peter Grünberg Institute 5, Forschungszentrum Jülich, 52425 Jülich, Germany*

(Dated: February 27, 2019)

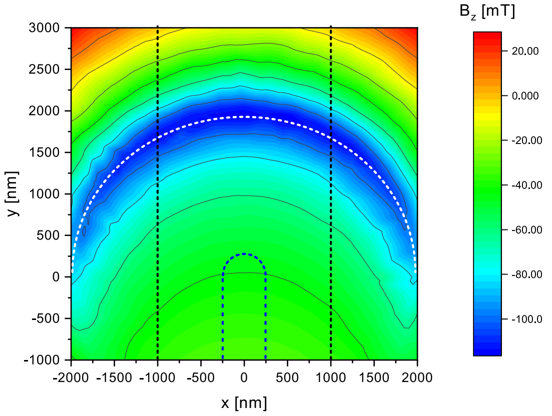


Figure S1. Finite element simulation of the magnetic field generated by the injection of a 350 mA current pulse across the Ω-shaped coil. The white dashed lines indicate the edges of the Ω-shaped coil, the black dashed lines indicate the edges of the microwire, and the blue dashed lines mark the edges of the skyrmion injector.

**Simulation of the magnetic field generated by the Ω-shaped microcoil**

The spatial distribution of the magnetic field generated by the Ω-shaped microcoil when annihilating the magnetic skyrmion was simulated with the commercial finite element multiphysics simulation suite ANSYS (see the Methods section for more details). The results of the simulations are shown in Fig. S1.

**Simulation of the current density distribution in the skyrmion injector**

The spatial distribution of the current density in the Pt/$Co_{68}B_{32}$/Ir microstructured wire when injecting a current pulse across the skyrmion injector was simulated once again using the commercial finite element multiphysics simulation suite ANSYS (see the Methods section for more details). The results of the simulations are shown in Fig. S2. It is possible to observe that a hot spot in the current density can be found at the tip of the skyrmion injector. In this point, a current density about a factor 3 higher than in the uniform section of the microwire can be observed.

It is also possible to observe that the elongated shape of the magnetic skyrmions nucleated in the time-resolved experiments presented in Figs. 4 and 5 of the main manuscript resembles the shape of the hot spot in the current density at the tip of the injector structure, suggesting

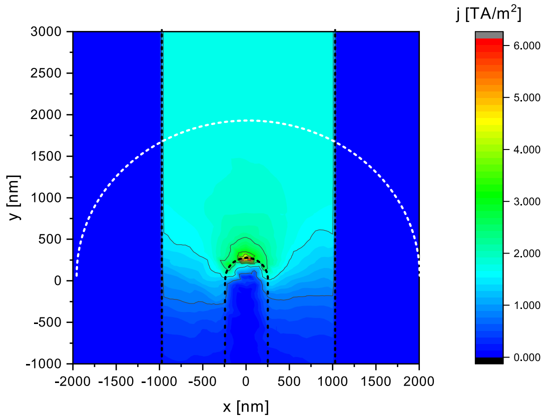


Figure S2. Finite element simulation of the spatial distribution of the current density in the Pt/$Co_{68}B_{32}$/Ir microwire when injecting a current pulse across the skyrmion injector. The white dashed lines indicate the edges of the Ω-shaped coil, while the black dashed lines indicate the edges of the microwire and of the skyrmion injector.

that the shape of the nucleated skyrmion could be controlled by tailoring the distribution of the injected current density at the tip of the skyrmion injector.

**Measurement of the dynamical temperature variation in the Pt/$Co_{68}B_{32}$/Ir multilayer stack**

The injection of a current pulse into the microwire causes its heating due to Ohmic losses. To determine the dynamical variation of the temperature of the Pt/$Co_{68}B_{32}$/Ir multilayer stack in the region where the skyrmion nucleation occurs, we measured the time-resolved variation of the saturation magnetization $M_s$ of the Pt/$Co_{68}B_{32}$/Ir multilayer stack. The time-resolved variation of $M_s$ was determined by measuring the variation in contrast in the uniformly magnetized region of the sample (see inset of Fig. S3). This measurement was normalized to the variation in magnetic contrast recorded in the region where the skyrmion is nucleated (where the magnetization switches completely). Under the assumption that the Pt/$Co_{68}B_{32}$/Ir multilayer stack remains perpendicularly magnetized during the injection of the current pulse, the time-resolved variation of $M_s$ calculated from the time-resolved images is shown in Fig. S3.

The time-resolved variation of the sample temperature was then determined by comparing the time-resolved variation of $M_s$ with the static variation of $M_s$ in the Pt/$Co_{68}B_{32}$/Ir multi-

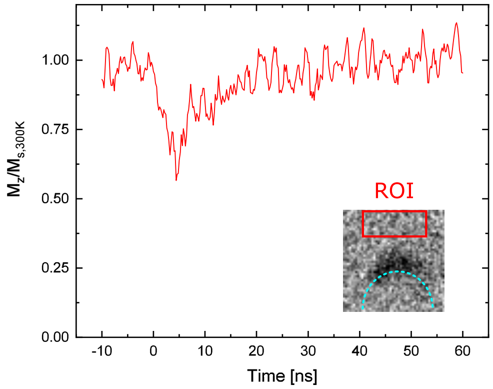


Figure S3. Time-resolved variation of the saturation magnetization (normalized to the saturation magnetization at room temperature) of the Pt/$Co_{68}B_{32}$/Ir multilayer stack in the region surrounding the skyrmion injector (area marked by ROI in the inset).

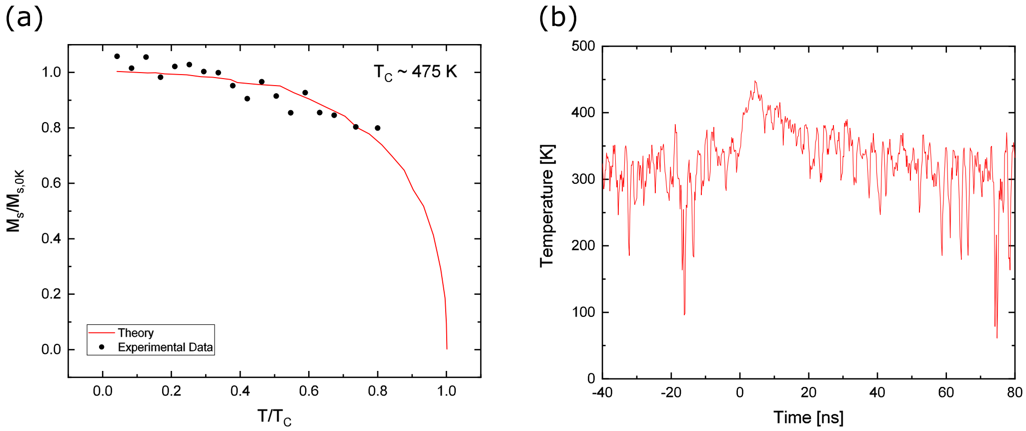


Figure S4. Comparison of the time-resolved variation in $M_s$ with the static dependence of $M_s$ as a function of the temperature. (a) Static dependence of $M_s$ as a function of the temperature, fitted to the expected dependence of $M_s(T)$. (b) Calculated time-resolved temperature of the Pt/$Co_{68}B_{32}$/Ir multilayer stack in the region surrounding the skyrmion injector.

layer stack as a function of the temperature, shown in Fig. S4(a), where a Curie temperature of about 475 K could be estimated for the Pt/$Co_{68}B_{32}$/Ir. The result of such calculation is shown in Fig. S4(b), where it is possible to observe that the maximum temperature after the injection of a 5 ns wide current pulse with a peak current density of $1.4 \times 10^{12}$ Am$^{-2}$ is of about 440 K.

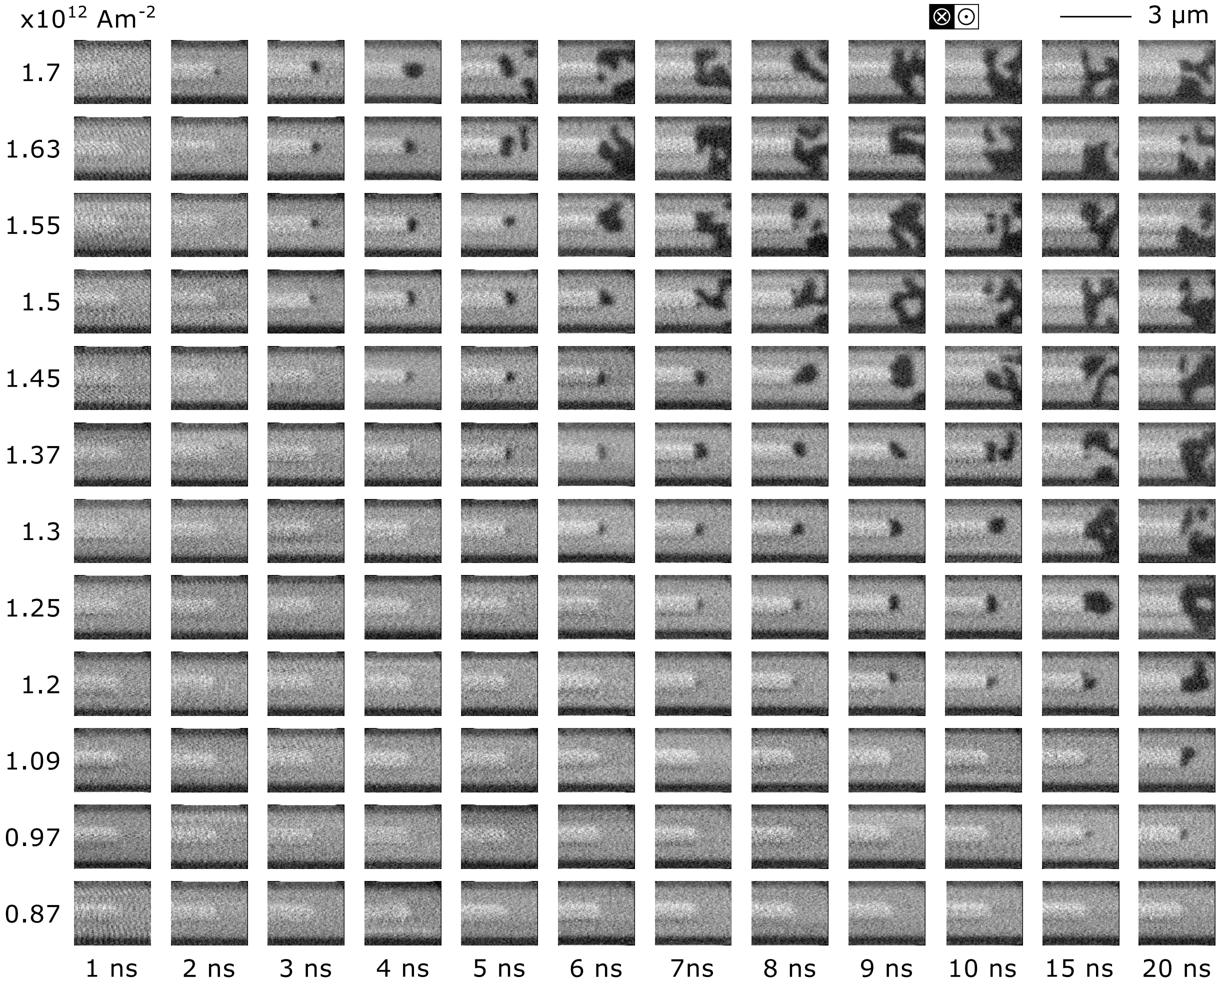


Figure S5. Quasi-static XMCD-STXM images of the skyrmion nucleation process as a function of pulse width and of the injected current density.

### XMCD-STXM images of the skyrmion nucleation process

In this section, the quasi-static XMCD-STXM images employed to obtain the results shown in Figs. 2 and 3 of the main manuscript are shown. A multidomain state was identified by the presence of either multiple domains in the field of view of the image, or by the presence of magnetic domains in contact with the edges of the microwire.

### Influence of the pulse characteristics on the skyrmion area

Here, the influence of the specifications of the current pulse injected in the Pt/$Co_{68}B_{32}$/Ir microwire on the area of the skyrmions nucleated by the pulse is shown. As described in

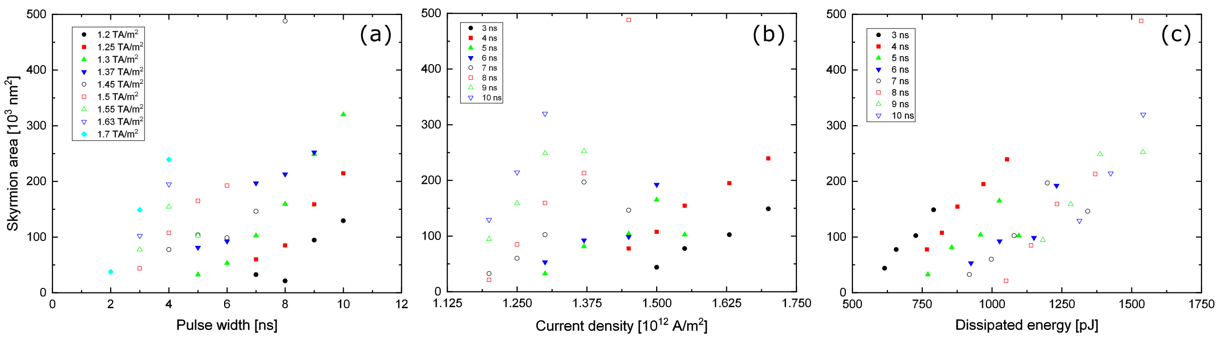


Figure S6. Dependence of the area of the magnetic skyrmions nucleated with a current pulse with respect to (a) the width of the current pulse (under equal current density), (b) the current density injected by the pulse (under equal pulse width), and on (c) the energy dissipated by the pulse (under equal pulse width).

the main manuscript, the increase of either the width or the current density of the injected pulse leads to an increase in the area of the nucleated magnetic skyrmion. A roughly linear dependence with either the width or the current density can be observed.

* Corresponding Author: simone.finizio@psi.ch
